# Supplementary material for: Optimization Methods and Software for Federated Learning
Source: arXiv:2509.08120 source file (2025-09-09)
Supplement: Supplementary file 1 [file Appendix_A.tex]

% Appendix A File

\refstepcounter{chapter}%
\chapter*{\thechapter \quad Appendix A Title}
\label{appendixA}

Detailed experimental procedures, data tables, and computer programs may be placed in appendices. This may be particularly appropriate if the dissertation or thesis includes several published papers.
