# Supplementary material for: Optimization Methods and Software for Federated Learning
Source: arXiv:2509.08120 source file (2025-09-09)
Supplement: Supplementary file 2 [file Appendix_B.tex]

% Appendix B File

\refstepcounter{chapter}%
\chapter*{\thechapter \quad Appendix B Title}
\label{appendixB}

Your content goes here.
